# Supplementary material for: MapPrior: Bird's-Eye View Map Layout Estimation with Generative Models
Source: arXiv:2308.12963 source file (2023-08-24)
Supplement: Supplementary file 1 [file architectures.tex]

\section{Model Architecture Details}

\label{sec:arch}
\paragraph{Predictive Stage} In the predictive stage, we are using BEVFusion\cite{bev_fusion}, with an unchanged model architecture. 
BEVFusion uses Swin-T\cite{liu2021swin} as the image backbone. It then applies FPN to fuse multi-scale camera features to produce a feature map of 1/8 input size. It downsamples camera images to 256×704. For the LiDAR backbone, BEVFusion adopts VoxelNet, using a voxel size of 0.1m. As a final step, BEVFusion uses a convolutional segmentation head to predict the BEV map.

\subsection{Auto-encoder}
We modified the model architecture from VQGAN\cite{VQGAN}. To make sure our input and output resolution of the BEV map is $200 \times 200$, and the latent space resolution is $12 \times 12$, we adjust the padding strategy in the auto-encoder model.

\paragraph{Encoder}
The encoder contains an input convolution layer followed by five downsampling blocks. Each downsampling block contains two res-net blocks. After downsampling, the encoder has two middle res-net blocks, one middle attention block, and one output convolution layer. We show detailed model architecture in Tab.~\ref{tab:Encoder}

\begin{table*}[!t]
\caption{Architecture for Encoder}
\begin{tabular}{|c|c|c|c|c|c|c|}
\hline
\multicolumn{2}{|c|}{layers} & \multicolumn{5}{|c|}{parameters} \\
\hline
input & Conv2d & \multicolumn{5}{|c|}{in\_ch:6, out\_ch: 128, kernel: 3x3, stride: 1, pad: 1 } \\
 \hline

\multirow{3}*{downsample\_block\_1} &  ResnetBlock & \multicolumn{5}{|c|}{in\_ch:128, out\_ch: 128 } \\
~ &  ResnetBlock & \multicolumn{5}{|c|}{in\_ch:128, out\_ch: 128 } \\
~ &  Downsample(Conv2d) & \multicolumn{5}{|c|}{in\_ch:128, out\_ch: 128,kernel:3x3, stride:2, padding=((0,1,0,1),val=0) } \\
\hline
\multirow{3}*{downsample\_block\_2} &  ResnetBlock & \multicolumn{5}{|c|}{in\_ch:128, out\_ch: 128 } \\
~ &  ResnetBlock & \multicolumn{5}{|c|}{in\_ch:128, out\_ch: 128 } \\
~ &  Downsample(Conv2d) & \multicolumn{5}{|c|}{in\_ch:128, out\_ch: 128,kernel:3x3, stride:2, padding=((0,1,0,1),val=0) } \\
\hline
\multirow{3}*{downsample\_block\_3} &  ResnetBlock & \multicolumn{5}{|c|}{in\_ch:128, out\_ch: 256 } \\
~ &  ResnetBlock & \multicolumn{5}{|c|}{in\_ch:256, out\_ch: 256 } \\
~ &  Downsample(Conv2d) & \multicolumn{5}{|c|}{in\_ch:256, out\_ch: 256,kernel:3x3, stride:2, padding=((0,1,0,1),val=0) } \\
\hline
\multirow{3}*{downsample\_block\_4} &  ResnetBlock & \multicolumn{5}{|c|}{in\_ch:256, out\_ch: 256 } \\
~ &  ResnetBlock & \multicolumn{5}{|c|}{in\_ch:256, out\_ch: 256 } \\
~ &  Downsample(Conv2d) & \multicolumn{5}{|c|}{in\_ch:256, out\_ch: 256,kernel:3x3, stride:2, padding=((0,1,0,1),val=0) } \\
\hline
\multirow{2}*{downsample\_block\_5} &  ResnetBlock & \multicolumn{5}{|c|}{in\_ch:256, out\_ch: 512 } \\
~ &  ResnetBlock & \multicolumn{5}{|c|}{in\_ch:256, out\_ch: 256 } \\

\hline
\multirow{3}*{middle} &  ResnetBlock & \multicolumn{5}{|c|}{in\_ch:512, out\_ch: 512 } \\
~ &  AttnBlock & \multicolumn{5}{|c|}{in\_ch:512 } \\
~ &  ResnetBlock & \multicolumn{5}{|c|}{in\_ch:512, out\_ch: 512 } \\
\hline
\multirow{3}*{end} &  Normalize & \multicolumn{5}{|c|}{GroupNorm,num\_groups=32, num\_channels=512} \\

~ &  Activation & \multicolumn{5}{|c|}{x*sigmoid(x)} \\

~ &  Conv2d & \multicolumn{5}{|c|}{in\_ch:512, out\_ch: 256, kernel: 3x3, stride: 1, pad: 1 } \\
\hline
\end{tabular}
\label{tab:Encoder}
\end{table*}

\paragraph{Codebook}
The codebook has 1024 different tokens, each of which is a 256-dimensional feature vector. Empirically we find this size trade-offs well between the generator's capacity and inference speed. 

\paragraph{Decoder}
The decoder has a similar structure as the encoder. It contains an input convolution layer, two res-net blocks, and one attention layer before the upsampling blocks. It then includes five upsampling blocks, each containing three res-net blocks. Finally, the decoder applies an output convolution layer. We show the detailed model architecture in Tab.~\ref{tab:decoder}

\begin{table*}[!t]
\caption{Architecture for Decoder}
\begin{tabular}{|c|c|c|c|c|c|c|}
\hline
\multicolumn{2}{|c|}{layers} & \multicolumn{5}{|c|}{parameters} \\
\hline
\multirow{1}*{input} & Conv2d & \multicolumn{5}{|c|}{in\_ch:256, out\_ch: 512, kernel: 3x3, stride: 1, pad: 1 } \\

\hline
\multirow{3}*{middle} &  ResnetBlock & \multicolumn{5}{|c|}{in\_ch:512, out\_ch: 512 } \\
~ &  AttnBlock & \multicolumn{5}{|c|}{in\_ch:512 } \\
~ &  ResnetBlock & \multicolumn{5}{|c|}{in\_ch:512, out\_ch: 512 } \\
\hline

\multirow{3}*{upsample\_block\_1} &  ResnetBlock & \multicolumn{5}{|c|}{in\_ch:512, out\_ch: 256 } \\
~ &  ResnetBlock & \multicolumn{5}{|c|}{in\_ch:256, out\_ch: 256 } \\
~ &  ResnetBlock & \multicolumn{5}{|c|}{in\_ch:256, out\_ch: 256 } \\
\hline
\multirow{5}*{upsample\_block\_2} &  ResnetBlock & \multicolumn{5}{|c|}{in\_ch:256, out\_ch: 256 } \\
~ &  ResnetBlock & \multicolumn{5}{|c|}{in\_ch:256, out\_ch: 256 } \\
~ &  ResnetBlock & \multicolumn{5}{|c|}{in\_ch:256, out\_ch: 256 } \\
~ &  Upsample(nearest\_interpolate) & \multicolumn{5}{|c|}{scale\_factor=2.0 } \\
~ &  Conv2d & \multicolumn{5}{|c|}{in\_ch:256, out\_ch: 256,kernel=3x3,stride=1,padding=1) } \\

\hline
\multirow{5}*{upsample\_block\_3} &  ResnetBlock & \multicolumn{5}{|c|}{in\_ch:256, out\_ch: 256 } \\
~ &  ResnetBlock & \multicolumn{5}{|c|}{in\_ch:256, out\_ch: 256 } \\
~ &  ResnetBlock & \multicolumn{5}{|c|}{in\_ch:256, out\_ch: 256 } \\
~ &  Upsample(nearest\_interpolate) & \multicolumn{5}{|c|}{scale\_factor=2.0 } \\
~ &  Conv2d & \multicolumn{5}{|c|}{in\_ch:256, out\_ch: 256,kernel=3x3,stride=1,padding=1) } \\

\hline
\multirow{5}*{upsample\_block\_4} &  ResnetBlock & \multicolumn{5}{|c|}{in\_ch:256, out\_ch: 128 } \\
~ &  ResnetBlock & \multicolumn{5}{|c|}{in\_ch:128, out\_ch: 128 } \\
~ &  ResnetBlock & \multicolumn{5}{|c|}{in\_ch:128, out\_ch: 128 } \\
~ &  Upsample(nearest\_interpolate) & \multicolumn{5}{|c|}{scale\_factor=2.0 } \\
~ &  Conv2d & \multicolumn{5}{|c|}{in\_ch:128, out\_ch: 128,kernel=3x3,stride=1,padding=1) } \\

\hline
\multirow{4}*{upsample\_block\_5} &  ResnetBlock & \multicolumn{5}{|c|}{in\_ch:128, out\_ch: 128 } \\
~ &  ResnetBlock & \multicolumn{5}{|c|}{in\_ch:128, out\_ch: 128 } \\
~ &  ResnetBlock & \multicolumn{5}{|c|}{in\_ch:128, out\_ch: 128 } \\
~ &  ConvTranspose2d & \multicolumn{5}{|c|}{in\_ch:128, out\_ch: 128, kennel:3x3,stride = 2} \\

\hline

\multirow{2}*{end} &  Normalize & \multicolumn{5}{|c|}{GroupNorm,num\_groups=32, num\_channels=512} \\
~ &  Conv2d & \multicolumn{5}{|c|}{in\_ch:128, out\_ch: 6, kernel: 3x3, stride: 1, pad: 1 } \\
\hline

\end{tabular}
\label{tab:decoder}
\end{table*}

\paragraph{Discriminator}
Following VQGAN, we define a 3-layer PatchGAN discriminator as in Pix2Pix \cite{pix2pix}. The discrimination takes the reconstructed output or the ground truth BEV map as input and outputs a prediction map to discriminate the reconstructed map from ground truth. It includes one input convolution layer using leaky ReLU as activation. It then includes three convolution layers with batch norm as normalization and leaky ReLU as activation. It finally contains an output convolution layer to output a one-channel prediction map.
 
\subsection{Latent Space Transformer}
The latent space transformer consists of a GPT transformer and a BEV feature extractor. The GPT transformer contains token embedding, feature embedding, and positional embedding. The token embedding is a learnable feature vector for each code in the codebook, and the positional embedding is a learnable feature vector for every position. The feature embedding is the output of the BEV feature extractor. The final embedding is the token embedding concatenated with feature embedding and then encoded with a positional embedding. The final embedding is then fed into 24 attention blocks, and each consists of one vanilla multi-head masked self-attention layer with 16 heads, three mlp layers, and layer norm. As in GPT, a causal mask ensures that attention is only applied to the past in the input sequence.

We present the detailed parameter of GPT in Tab.~\ref{tab:transformer}. The BEV feature extractor shares a similar architecture as the encoder. We present the detailed architecture in Tab. ~\ref{tab:feature}.

\begin{table}[h] \centering
\caption{Architecture for Transformer}
\begin{tabular}{|c|c|}
\hline
parameters & value \\
\hline
vocab\_size & 1024 \\
\hline
block\_size(context\_size) & 512 \\
\hline
n\_layer & 24 \\
\hline
n\_head & 16 \\
\hline
n\_embd & 1024\\
\hline
\end{tabular}
\label{tab:transformer}

\end{table}

\begin{table*}[!t]
\caption{Architecture for BEV Feature Extarctor}
\begin{tabular}{|c|c|c|c|c|c|c|}
\hline
\multicolumn{2}{|c|}{layers} & \multicolumn{5}{|c|}{parameters} \\
\hline
input & Conv2d & \multicolumn{5}{|c|}{in\_ch:80/256, out\_ch: 128, kernel: 3x3, stride: 1, pad: 1 } \\
\hline

\multirow{3}*{downsample\_block\_1} &  ResnetBlock & \multicolumn{5}{|c|}{in\_ch:128, out\_ch: 128 } \\
~ &  ResnetBlock & \multicolumn{5}{|c|}{in\_ch:128, out\_ch: 128 } \\
~ &  Downsample(Conv2d) & \multicolumn{5}{|c|}{in\_ch:128, out\_ch: 128,kernel:3x3, stride:2, padding=((0,1,0,1),val=0) } \\
\hline
\multirow{3}*{downsample\_block\_2} &  ResnetBlock & \multicolumn{5}{|c|}{in\_ch:128, out\_ch: 128 } \\
~ &  ResnetBlock & \multicolumn{5}{|c|}{in\_ch:128, out\_ch: 128 } \\
~ &  Downsample(Conv2d) & \multicolumn{5}{|c|}{in\_ch:128, out\_ch: 128,kernel:3x3, stride:2, padding=((0,1,0,1),val=0) } \\
\hline
\multirow{3}*{downsample\_block\_3} &  ResnetBlock & \multicolumn{5}{|c|}{in\_ch:128, out\_ch: 256 } \\
~ &  ResnetBlock & \multicolumn{5}{|c|}{in\_ch:256, out\_ch: 256 } \\
~ &  Downsample(Conv2d) & \multicolumn{5}{|c|}{in\_ch:256, out\_ch: 256,kernel:3x3, stride:2, padding=((0,1,0,1),val=0) } \\
\hline
\multirow{2}*{downsample\_block\_4} &  ResnetBlock & \multicolumn{5}{|c|}{in\_ch:256, out\_ch: 512 } \\
~ &  ResnetBlock & \multicolumn{5}{|c|}{in\_ch:256, out\_ch: 256 } \\
\hline
\multirow{3}*{middle} &  ResnetBlock & \multicolumn{5}{|c|}{in\_ch:512, out\_ch: 512 } \\
~ &  AttnBlock & \multicolumn{5}{|c|}{in\_ch:512 } \\
~ &  ResnetBlock & \multicolumn{5}{|c|}{in\_ch:512, out\_ch: 512 } \\
\hline
\multirow{3}*{end} &  Normalize & \multicolumn{5}{|c|}{GroupNorm,num\_groups=32, num\_channels=512} \\

~ &  Activation & \multicolumn{5}{|c|}{x*sigmoid(x)} \\

~ &  Conv2d & \multicolumn{5}{|c|}{in\_ch:512, out\_ch: 256, kernel: 3x3, stride: 1, pad: 1} \\
\hline

\end{tabular}
\label{tab:feature}
\end{table*}
