# Supplementary material for: MapPrior: Bird's-Eye View Map Layout Estimation with Generative Models
Source: arXiv:2308.12963 source file (2023-08-24)
Supplement: Supplementary file 2 [file qual.tex]

\section{Additional Qualitative Results}
\label{sec:qual}
\subsection{Map Segmentation as Generation}

We provide additional Qualitative results for BEV map segmentation in Fig.~\ref{Additional_qual_L1} \ref{Additional_qual_L2} \ref{Additional_qual_C1} \ref{Additional_qual_C2}. The figures show that our model consistently generates results with better accuracy and realism than the baseline.  For instance, the fourth row of Fig.~\ref{Additional_qual_L1} demonstrates our approach preserves a realistic layout of a complicated multi-way intersection, with straight and complete lane boundaries, well-structured cross-walks as well as complete sidewalks, while the baseline's estimate is significantly noisier. In addition, the first row of Fig.~\ref{Additional_qual_L2} demonstrates our approach can complete the vertical layout of the road at the intersection despite limited sensor input. The generated vertical layout also preserves a realistic layout with well-structured lanes, crosswalks, and sidewalks. For another example, the first row in Fig.~\ref{Additional_qual_C2} demonstrates our approach generates correct and regular spacing of the lane boundaries, as well as smoother boundaries of sidewalks and roads than the camera baseline.

In addition, we provide more diversity and uncertainty calibration results in Fig.~\ref{Additional Sampling Diversity} and ~\ref{Additional_Uncertainty Calibration}. Fig.~\ref{Additional Sampling Diversity} demonstrates that MapPrior can generate multiple diverse results, which can be aggregated into an accurate uncertainty map. Fig.~\ref{Additional_Uncertainty Calibration} shows that MapPrior's uncertainty map aligns better with the error map in different scenes.

 \begin{figure*}[!t] \centering 
 \begin{tabular}{ccccc} \centering
 \includegraphics[width=0.19\textwidth]{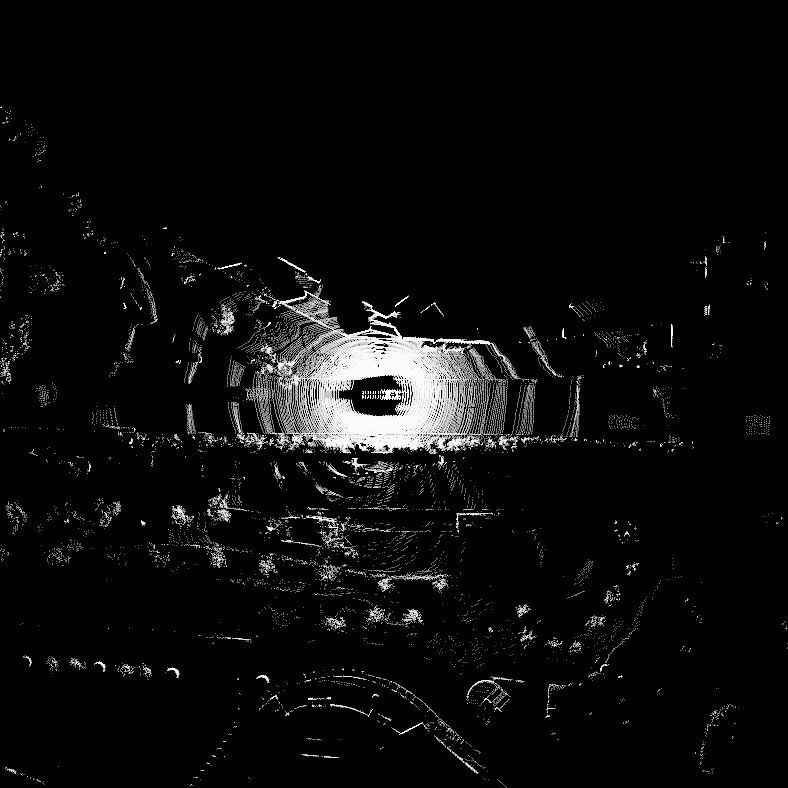}
 &\includegraphics[width=0.19\textwidth]{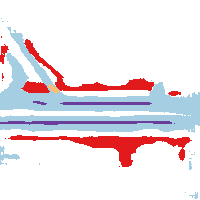}
 &\includegraphics[width=0.19\textwidth]{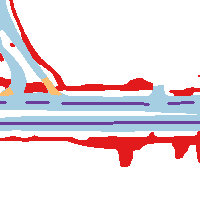}
&\includegraphics[width=0.19\textwidth]{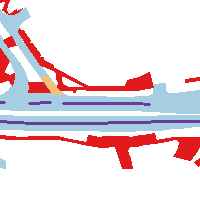}
\\
 \includegraphics[width=0.19\textwidth]{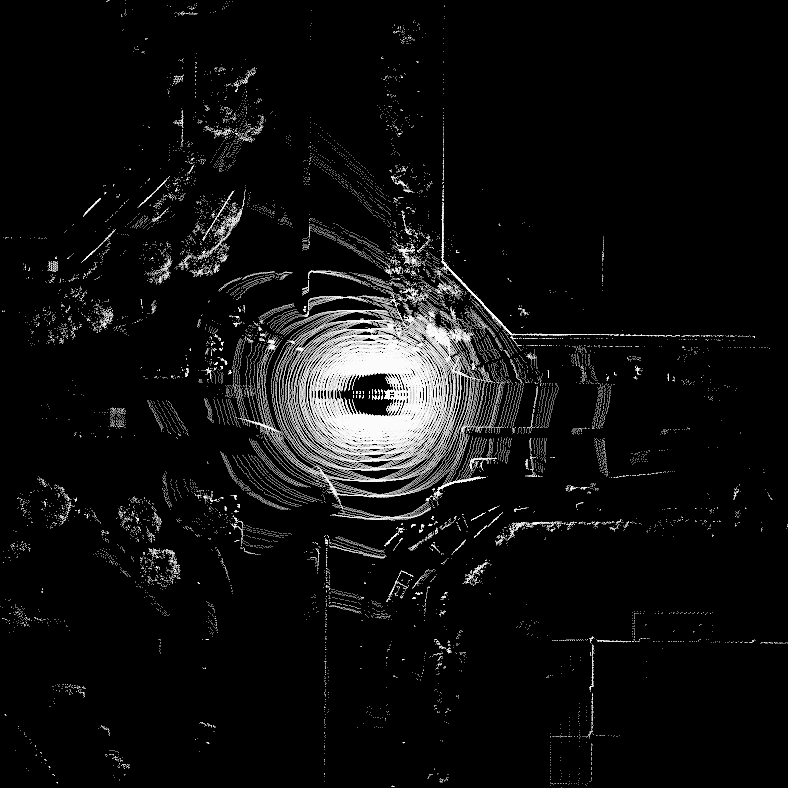}
 &\includegraphics[width=0.19\textwidth]{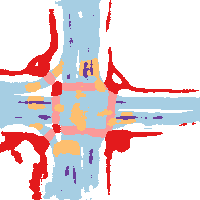}
 &\includegraphics[width=0.19\textwidth]{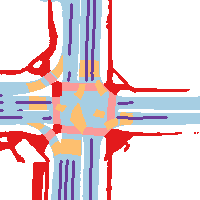}
&\includegraphics[width=0.19\textwidth]{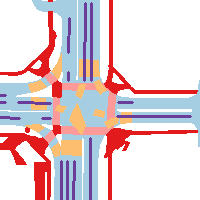}
\\
 \includegraphics[width=0.19\textwidth]{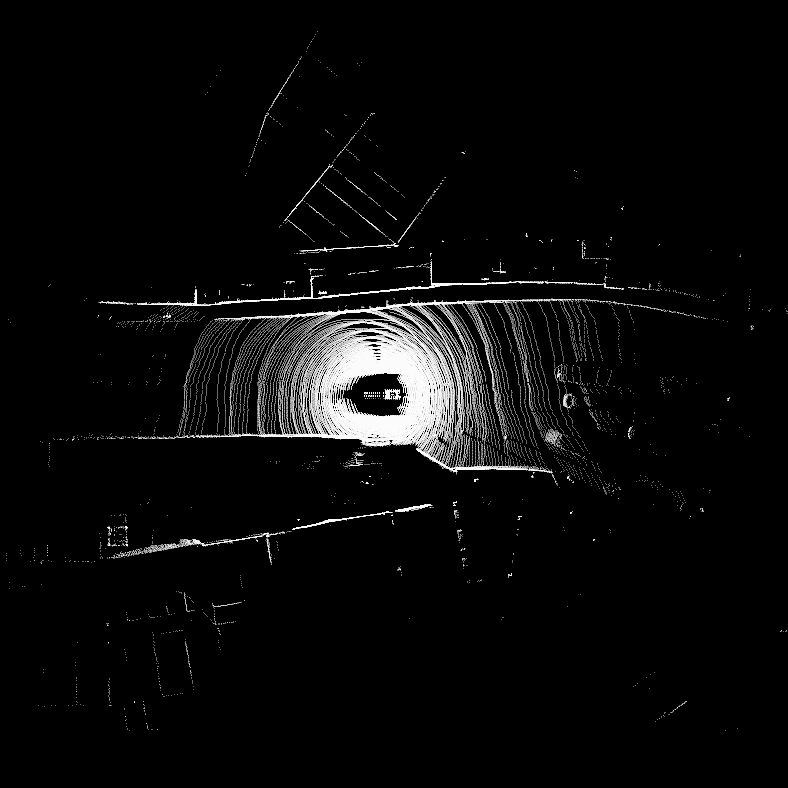}
 &\includegraphics[width=0.19\textwidth]{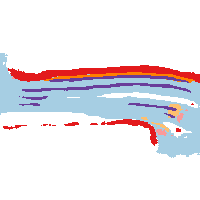}
 &\includegraphics[width=0.19\textwidth]{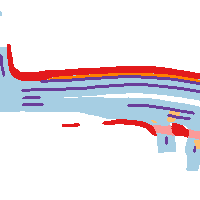}
&\includegraphics[width=0.19\textwidth]{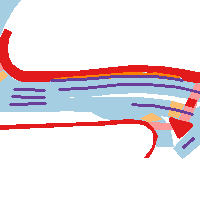}
\\
 \includegraphics[width=0.19\textwidth]{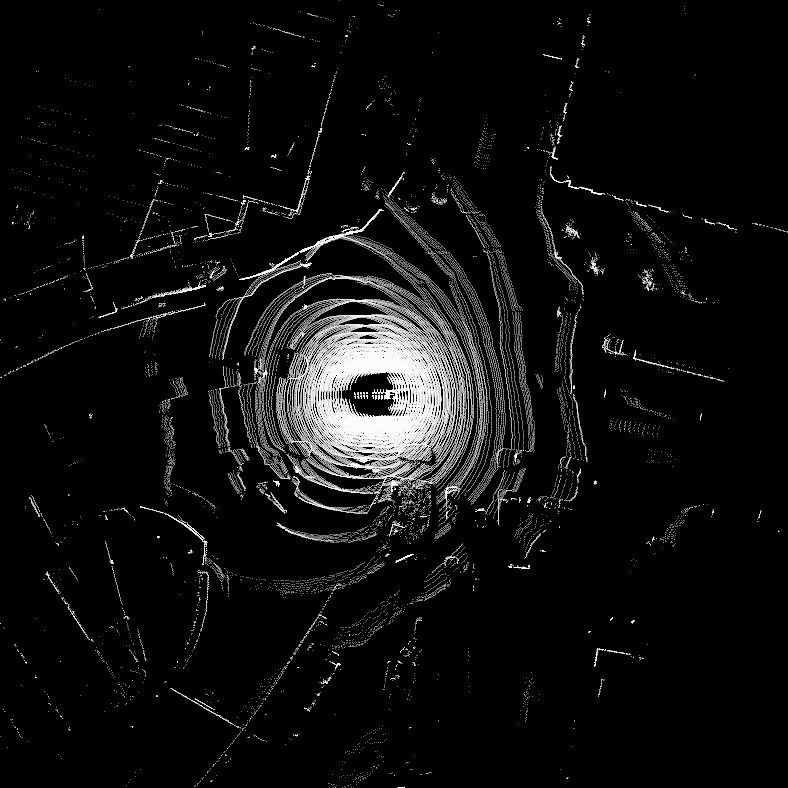}
 &\includegraphics[width=0.19\textwidth]{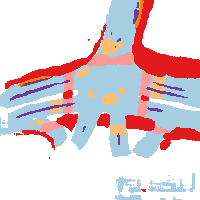}
 &\includegraphics[width=0.19\textwidth]{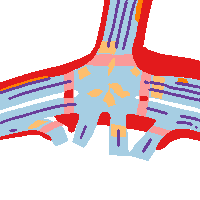}
&\includegraphics[width=0.19\textwidth]{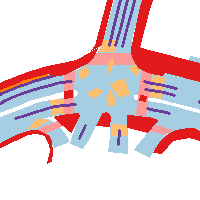}
\\
 \includegraphics[width=0.19\textwidth]{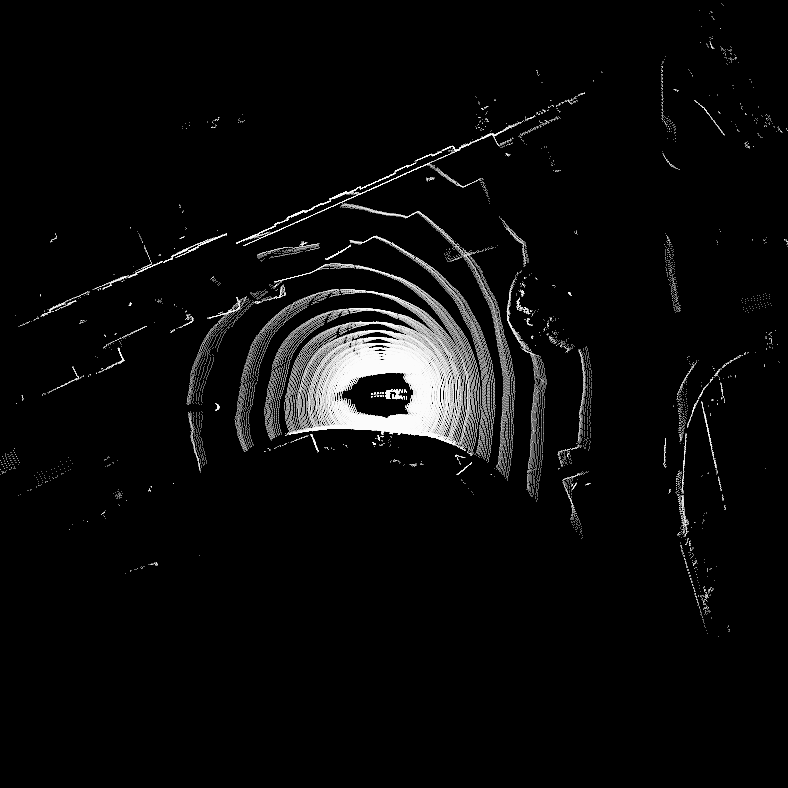}
 &\includegraphics[width=0.19\textwidth]{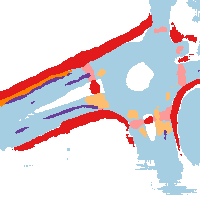}
 &\includegraphics[width=0.19\textwidth]{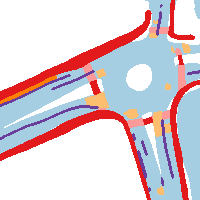}
&\includegraphics[width=0.19\textwidth]{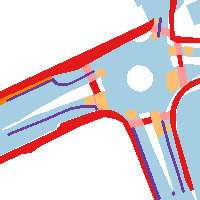}
\\
 \includegraphics[width=0.19\textwidth]{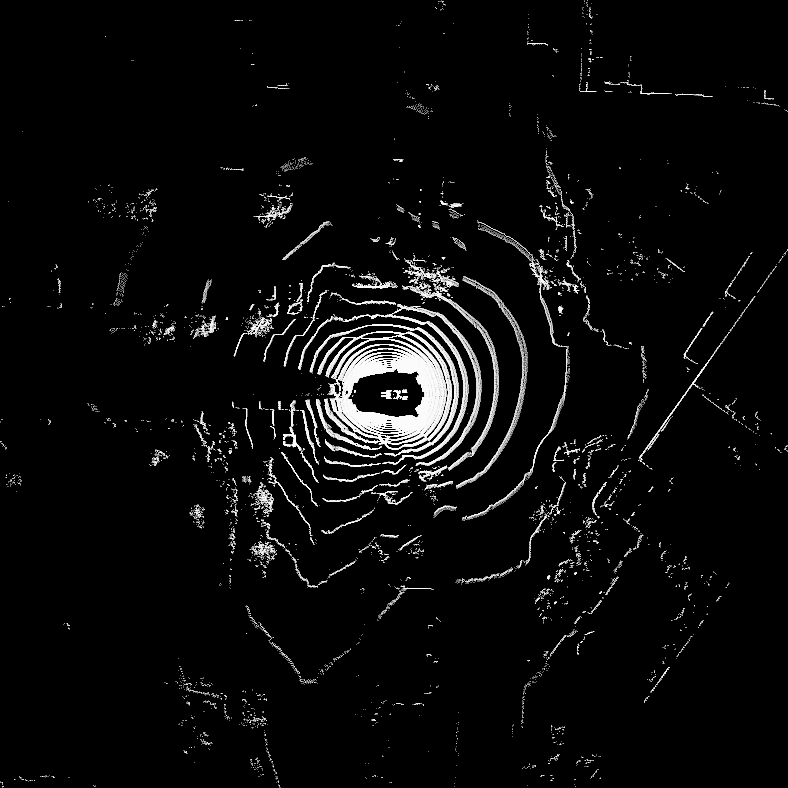}
 &\includegraphics[width=0.19\textwidth]{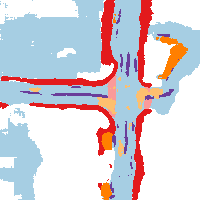}
 &\includegraphics[width=0.19\textwidth]{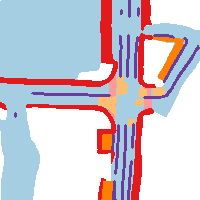}
&\includegraphics[width=0.19\textwidth]{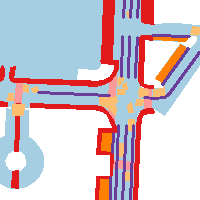}
\\

Input & BEVFusion-L & MapPrior-L (Ours) & GT
 \end{tabular}
 \caption{Additional results of BEV map segmentation on
nuScenes}

 \label{Additional_qual_L1}
 \vspace{-4pt}
 \end{figure*}

 \begin{figure*}[!t] \centering 
 \begin{tabular}{ccccc} \centering

 \includegraphics[width=0.19\textwidth]{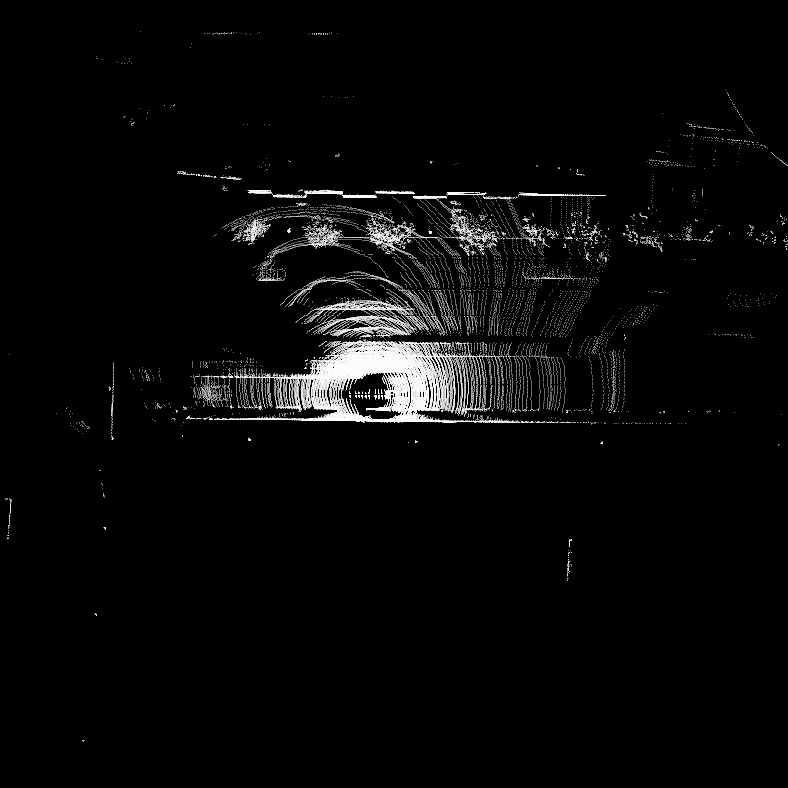}
 &\includegraphics[width=0.19\textwidth]{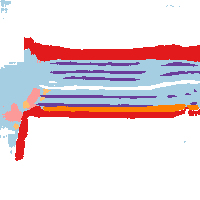}
 &\includegraphics[width=0.19\textwidth]{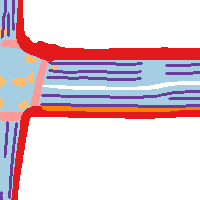}
&\includegraphics[width=0.19\textwidth]{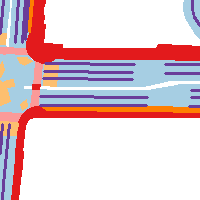}
\\
 \includegraphics[width=0.19\textwidth]{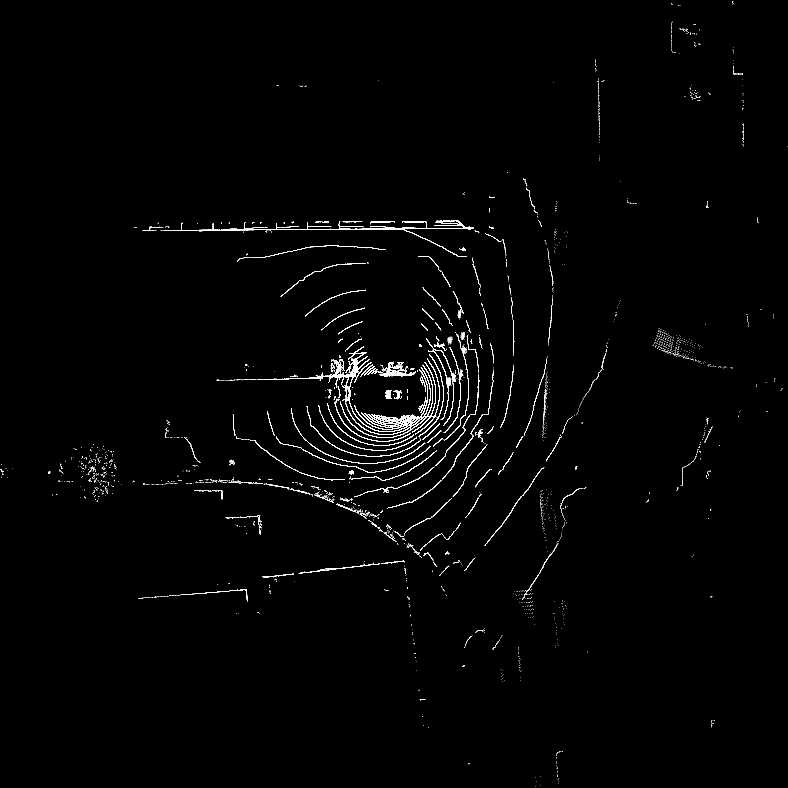}
 &\includegraphics[width=0.19\textwidth]{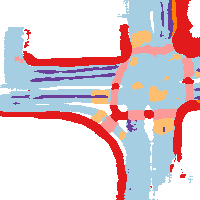}
 &\includegraphics[width=0.19\textwidth]{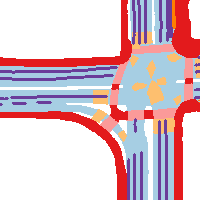}
&\includegraphics[width=0.19\textwidth]{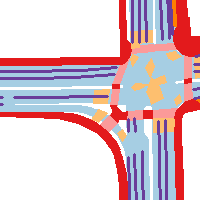}
\\
 \includegraphics[width=0.19\textwidth]{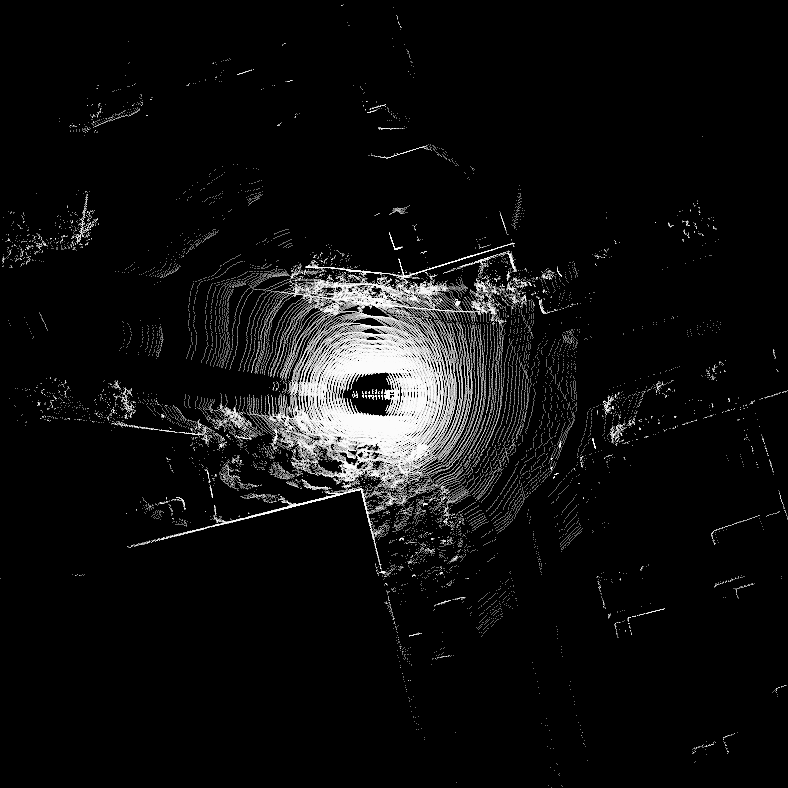}
 &\includegraphics[width=0.19\textwidth]{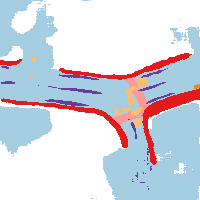}
 &\includegraphics[width=0.19\textwidth]{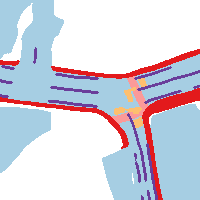}
&\includegraphics[width=0.19\textwidth]{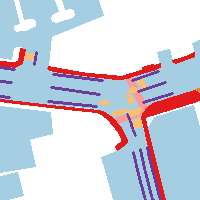}
\\
 \includegraphics[width=0.19\textwidth]{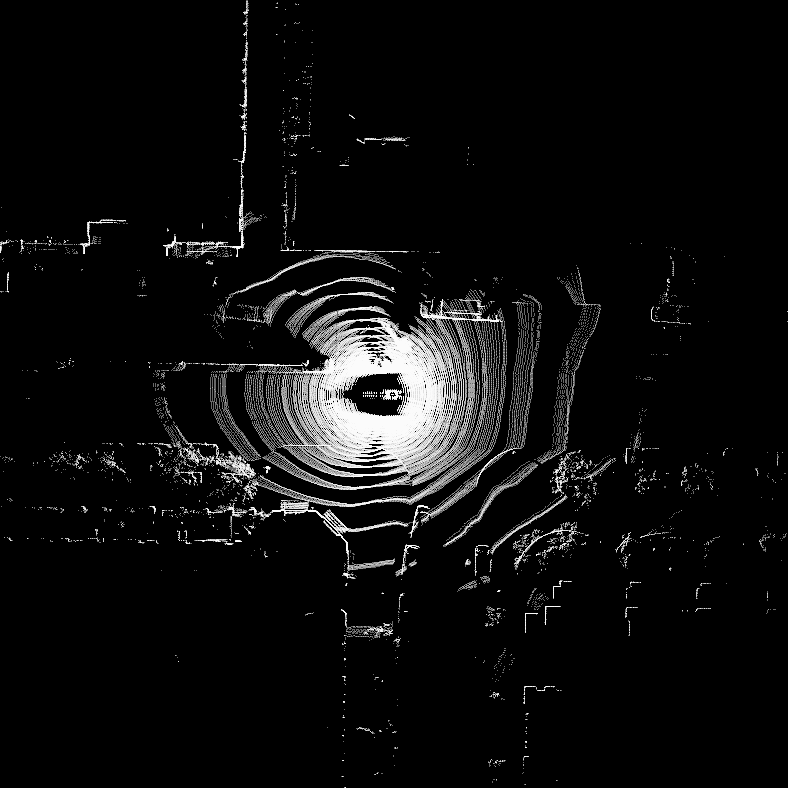}
 &\includegraphics[width=0.19\textwidth]{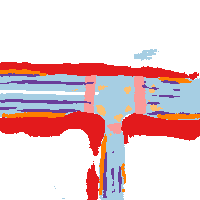}
 &\includegraphics[width=0.19\textwidth]{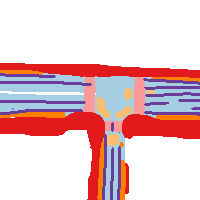}
&\includegraphics[width=0.19\textwidth]{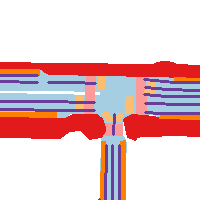}
\\
 \includegraphics[width=0.19\textwidth]{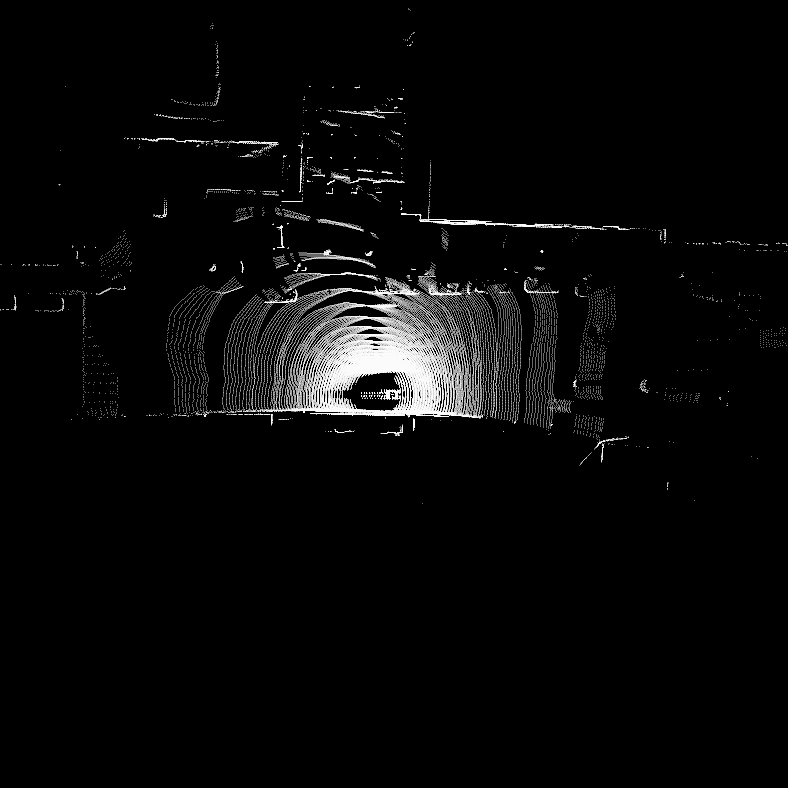}
 &\includegraphics[width=0.19\textwidth]{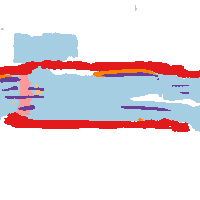}
 &\includegraphics[width=0.19\textwidth]{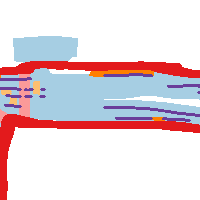}
&\includegraphics[width=0.19\textwidth]{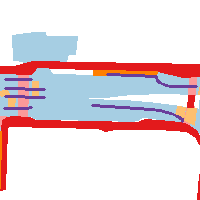}
\\
 \includegraphics[width=0.19\textwidth]{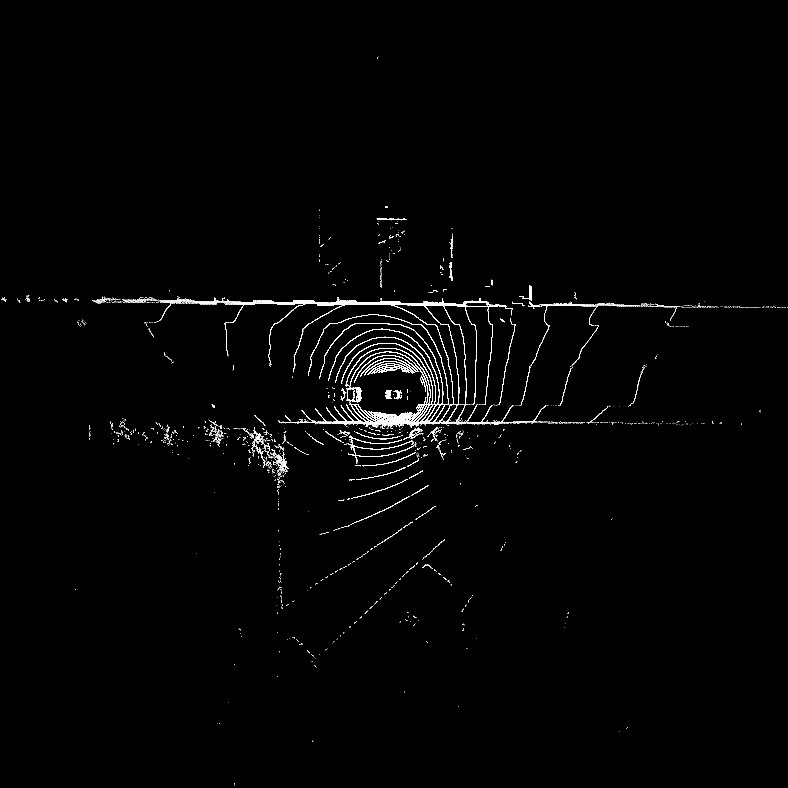}
 &\includegraphics[width=0.19\textwidth]{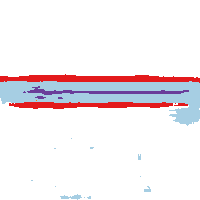}
 &\includegraphics[width=0.19\textwidth]{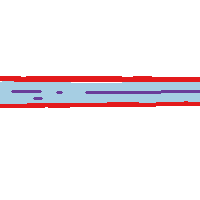}
&\includegraphics[width=0.19\textwidth]{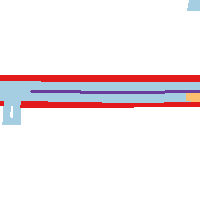}
\\
Input & BEVFusion-L & MapPrior-L (Ours) & GT
 \end{tabular}
 \caption{Additional Lidar results of BEV map segmentation on
nuScenes, continued}
 \label{Additional_qual_L2}
 \vspace{-4pt}
 \end{figure*}

 \begin{figure*}[!t] \centering 
 \begin{tabular}{ccccc} \centering
 \includegraphics[width=0.19\textwidth]{fig/more_samples/C/camera_order_2002.png}
 &\includegraphics[width=0.19\textwidth]{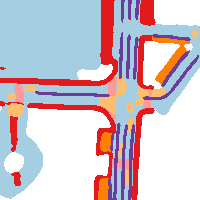}
 &\includegraphics[width=0.19\textwidth]{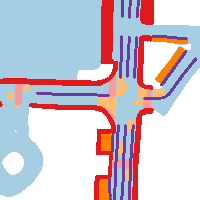}
&\includegraphics[width=0.19\textwidth]{fig/more_samples/GT/gt_2002.png}
\\
 \includegraphics[width=0.19\textwidth]{fig/more_samples/C/camera_order_2022.png}
 &\includegraphics[width=0.19\textwidth]{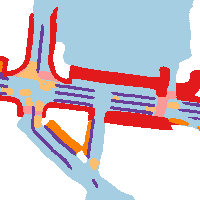}
 &\includegraphics[width=0.19\textwidth]{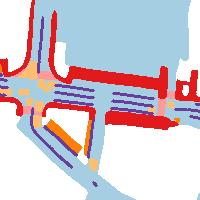}
&\includegraphics[width=0.19\textwidth]{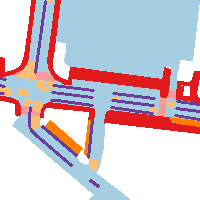}
\\
 \includegraphics[width=0.19\textwidth]{fig/more_samples/C/camera_order_2302.png}
 &\includegraphics[width=0.19\textwidth]{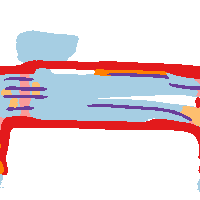}
 &\includegraphics[width=0.19\textwidth]{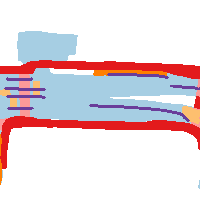}
&\includegraphics[width=0.19\textwidth]{fig/more_samples/GT/gt_2302.png}
\\
 \includegraphics[width=0.19\textwidth]{fig/more_samples/C/camera_order_2602.png}
 &\includegraphics[width=0.19\textwidth]{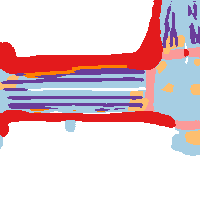}
 &\includegraphics[width=0.19\textwidth]{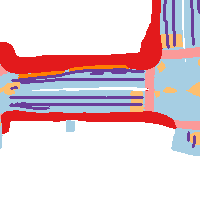}
&\includegraphics[width=0.19\textwidth]{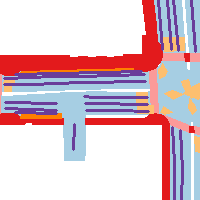}
\\
 \includegraphics[width=0.19\textwidth]{fig/more_samples/C/camera_order_2502.png}
 &\includegraphics[width=0.19\textwidth]{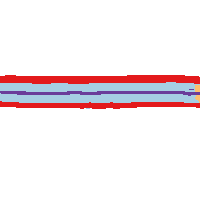}
 &\includegraphics[width=0.19\textwidth]{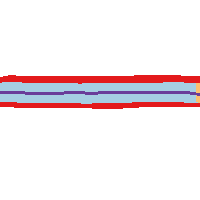}
&\includegraphics[width=0.19\textwidth]{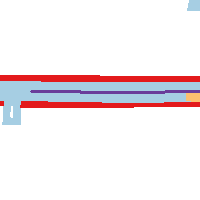}
\\
 \includegraphics[width=0.19\textwidth]{fig/more_samples/C/camera_order_2562.png}
 &\includegraphics[width=0.19\textwidth]{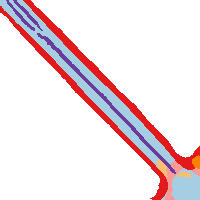}
 &\includegraphics[width=0.19\textwidth]{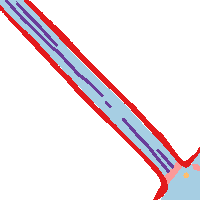}
&\includegraphics[width=0.19\textwidth]{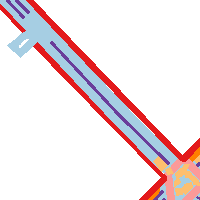}
\\
Input & BEVFusion-C & MapPrior-L (Ours) & GT
 \end{tabular}
 \caption{Additional Camera results of BEV map segmentation on
nuScenes}

 \label{Additional_qual_C1}
 \vspace{-4pt}
 \end{figure*}

 \begin{figure*}[!t] \centering 
 \begin{tabular}{ccccc} \centering
 \includegraphics[width=0.19\textwidth]{fig/more_samples/C/camera_order_2142.png}
 &\includegraphics[width=0.19\textwidth]{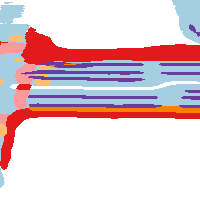}
 &\includegraphics[width=0.19\textwidth]{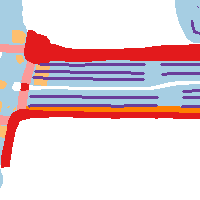}
&\includegraphics[width=0.19\textwidth]{fig/more_samples/GT/gt_2142.png}
\\
 \includegraphics[width=0.19\textwidth]{fig/more_samples/C/camera_order_2042.png}
 &\includegraphics[width=0.19\textwidth]{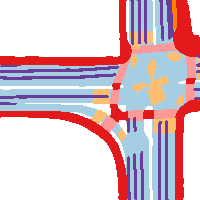}
 &\includegraphics[width=0.19\textwidth]{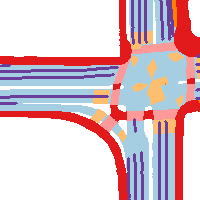}
&\includegraphics[width=0.19\textwidth]{fig/more_samples/GT/gt_2042.png}
\\
 \includegraphics[width=0.19\textwidth]{fig/more_samples/C/camera_order_2362.png}
 &\includegraphics[width=0.19\textwidth]{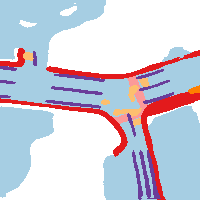}
 &\includegraphics[width=0.19\textwidth]{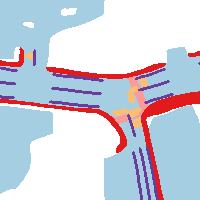}
&\includegraphics[width=0.19\textwidth]{fig/more_samples/GT/gt_2362.png}
\\
 \includegraphics[width=0.19\textwidth]{fig/more_samples/C/camera_order_2202.png}
 &\includegraphics[width=0.19\textwidth]{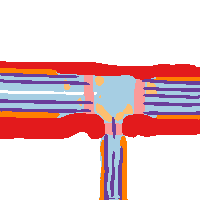}
 &\includegraphics[width=0.19\textwidth]{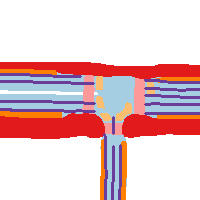}
&\includegraphics[width=0.19\textwidth]{fig/more_samples/GT/gt_2202.png}
\\
 \includegraphics[width=0.19\textwidth]{fig/more_samples/C/camera_order_2302.png}
 &\includegraphics[width=0.19\textwidth]{fig/more_samples/C/nos_2302.png}
 &\includegraphics[width=0.19\textwidth]{fig/more_samples/C/res_2302.png}
&\includegraphics[width=0.19\textwidth]{fig/more_samples/GT/gt_2302.png}
\\
 \includegraphics[width=0.19\textwidth]{fig/more_samples/C/camera_order_2402.png}
 &\includegraphics[width=0.19\textwidth]{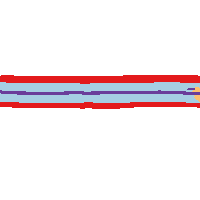}
 &\includegraphics[width=0.19\textwidth]{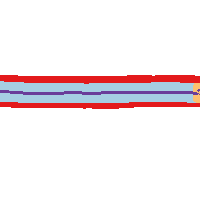}
&\includegraphics[width=0.19\textwidth]{fig/more_samples/GT/gt_2402.png}
\\
Input & BEVFusion-C & MapPrior-C (Ours) & GT
 \end{tabular}
 \caption{Additional Camera results of BEV map segmentation on
nuScenes, continued}

 \label{Additional_qual_C2}
 \vspace{-4pt}
 \end{figure*}

 \begin{figure*}[b] \centering 
 \begin{tabular}{cccccc} \centering
 \includegraphics[width=0.15\textwidth]{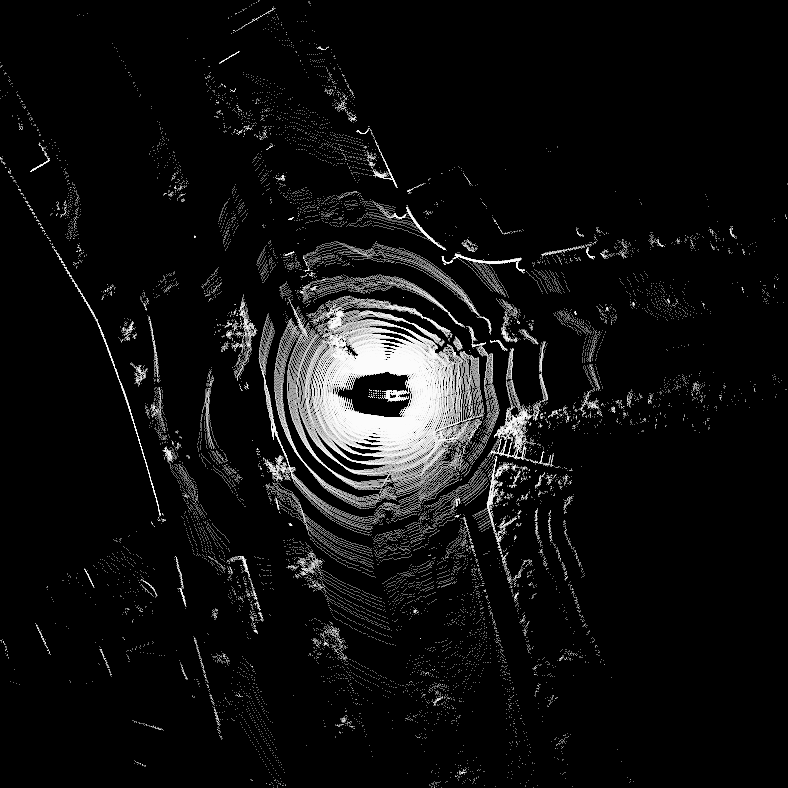}
 &\includegraphics[width=0.15\textwidth]{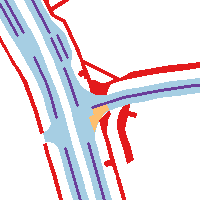}
 &\includegraphics[width=0.15\textwidth]{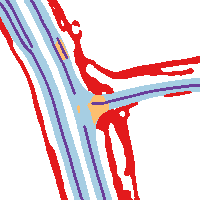}
&\includegraphics[width=0.15\textwidth]{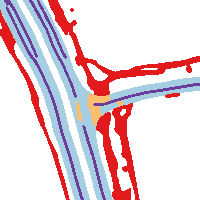}
&\includegraphics[width=0.15\textwidth]{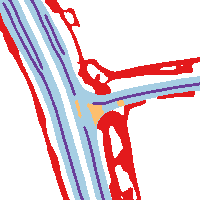}
&\includegraphics[width=0.15\textwidth]{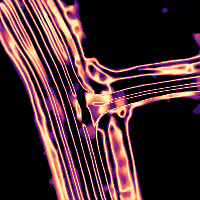} 
\\
 \includegraphics[width=0.15\textwidth]{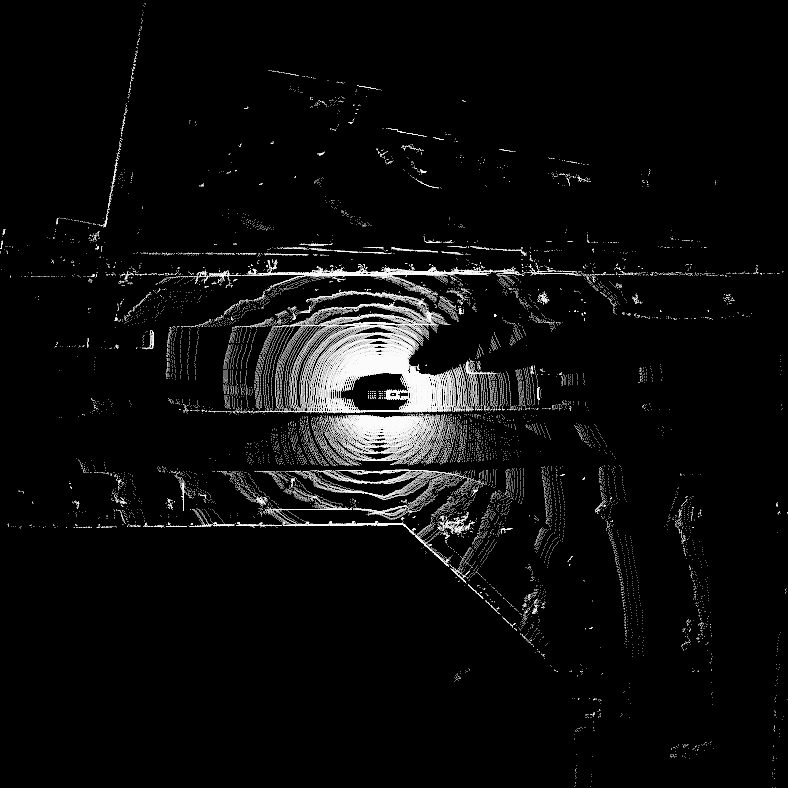}
 &\includegraphics[width=0.15\textwidth]{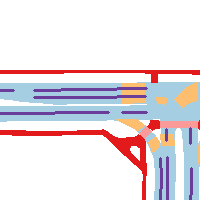}
 &\includegraphics[width=0.15\textwidth]{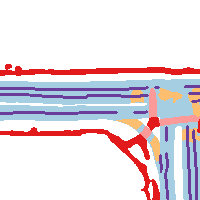}
&\includegraphics[width=0.15\textwidth]{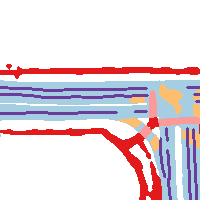}
&\includegraphics[width=0.15\textwidth]{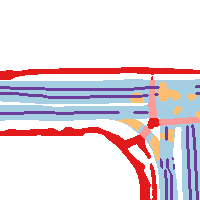}
&\includegraphics[width=0.15\textwidth]{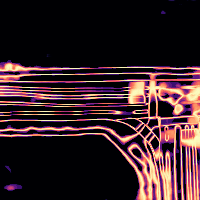} 
\\

\includegraphics[width=0.15\textwidth]{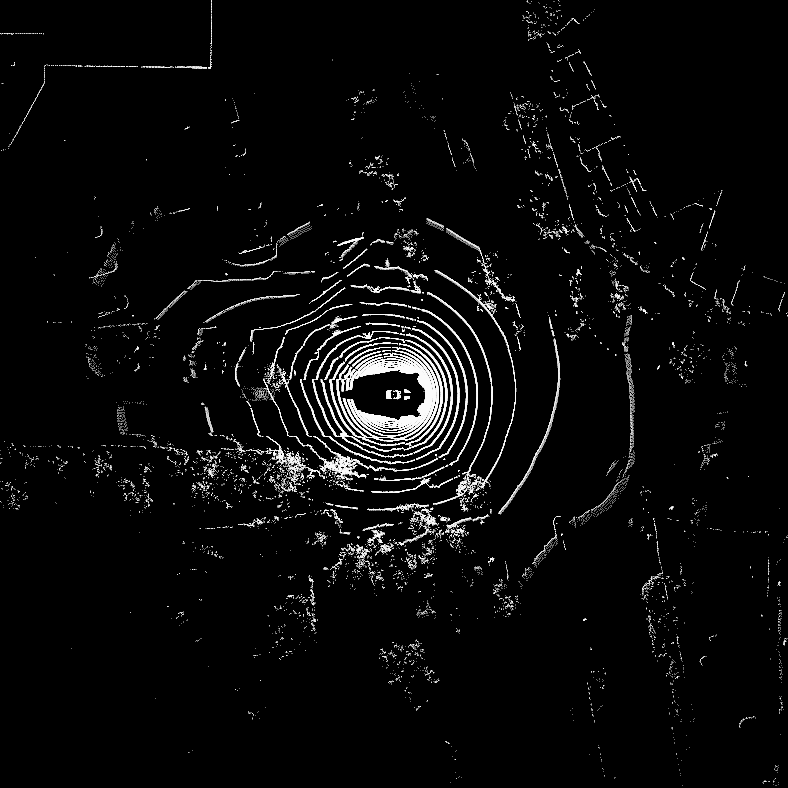}
 &\includegraphics[width=0.15\textwidth]{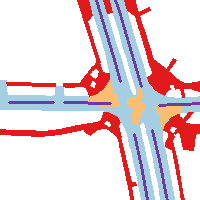}
 &\includegraphics[width=0.15\textwidth]{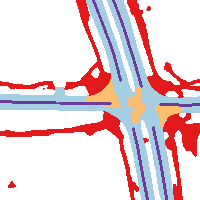}
&\includegraphics[width=0.15\textwidth]{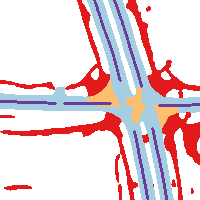}
&\includegraphics[width=0.15\textwidth]{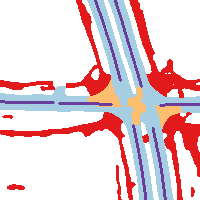}
&\includegraphics[width=0.15\textwidth]{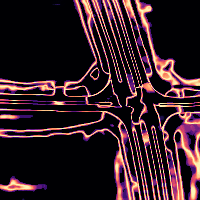}
\\
Input & GT & Our Sample 1 & Our Sample 2 & Our Sample 3 &  Uncertainty Map
 \end{tabular}
 \caption{Additional Qualitative results of diversity on NuScenes.}

 \label{Additional Sampling Diversity}
 \vspace{-4pt}
 \end{figure*}

 \begin{figure*}[b] \centering 
 \begin{tabular}{ccccccc} \centering

\includegraphics[width=0.12\textwidth]{fig/diverse_res/lidar_42.png} &
 \includegraphics[width=0.12\textwidth]{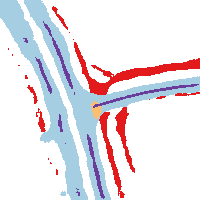} &  
 \includegraphics[width=0.12\textwidth]{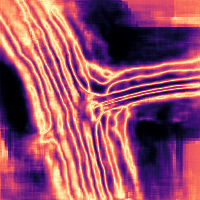} & 
 \includegraphics[width=0.12\textwidth]{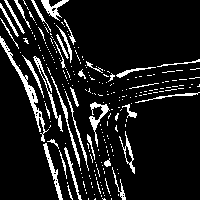} & 
 \includegraphics[width=0.12\textwidth]{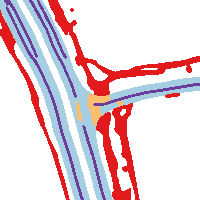} &  
 \includegraphics[width=0.12\textwidth]{fig/diverse_res/res_uncertainty42.png} &
  \includegraphics[width=0.12\textwidth]{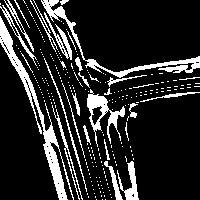} \\
  
\includegraphics[width=0.12\textwidth]{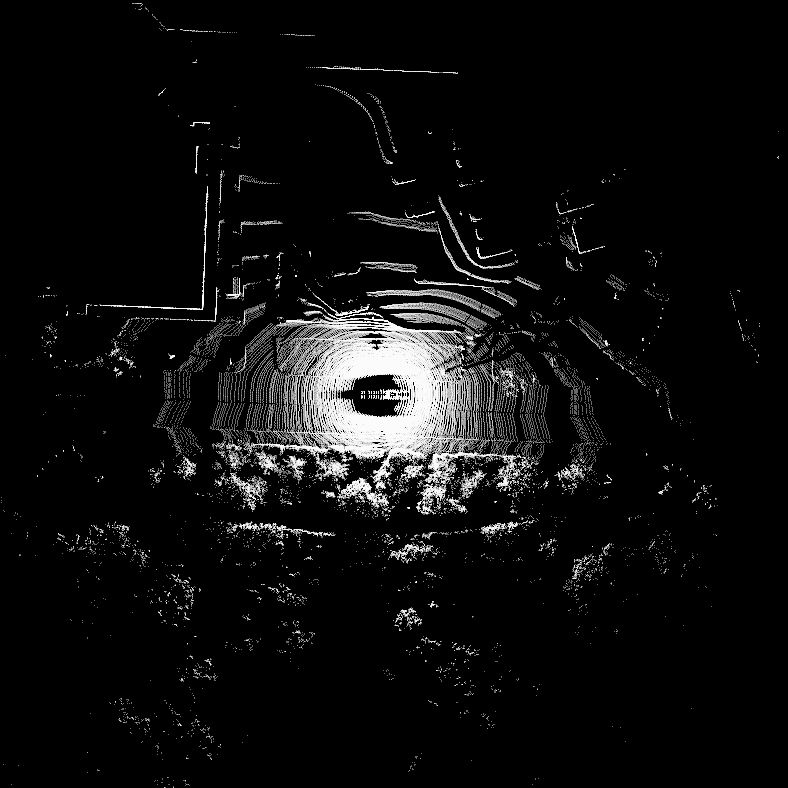} & 
 \includegraphics[width=0.12\textwidth]{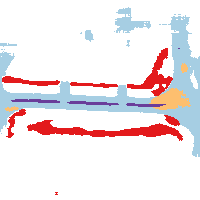} &  
 \includegraphics[width=0.12\textwidth]{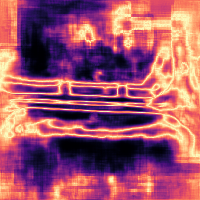} & 
 \includegraphics[width=0.12\textwidth]{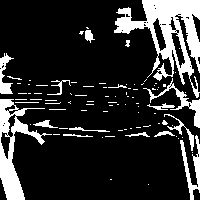} & 
 \includegraphics[width=0.12\textwidth]{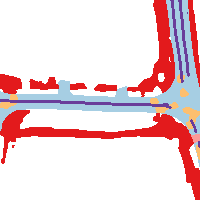} &  
 \includegraphics[width=0.12\textwidth]{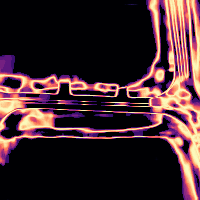} &
  \includegraphics[width=0.12\textwidth]{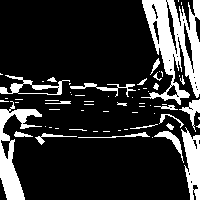} \\
 
\includegraphics[width=0.12\textwidth]{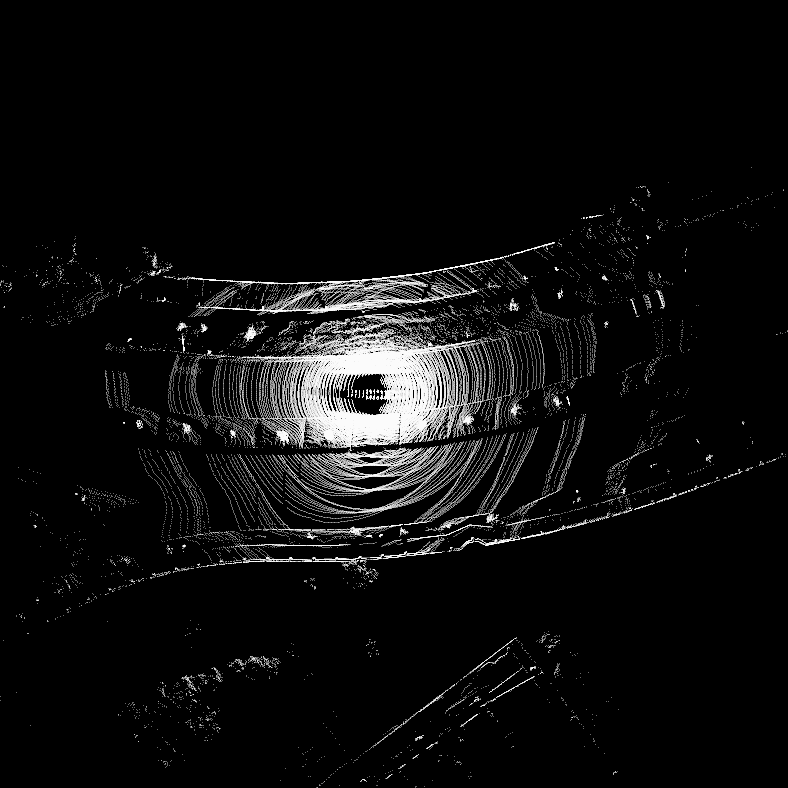} & 
 \includegraphics[width=0.12\textwidth]{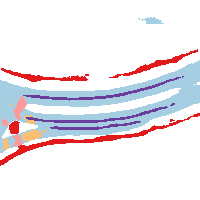} &  
 \includegraphics[width=0.12\textwidth]{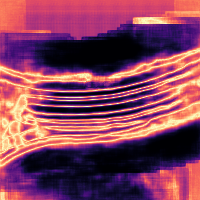} & 
 \includegraphics[width=0.12\textwidth]{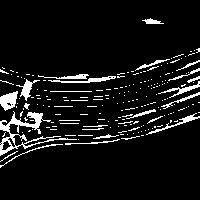} & 
 \includegraphics[width=0.12\textwidth]{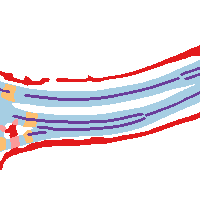} &  
 \includegraphics[width=0.12\textwidth]{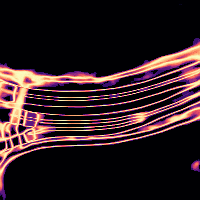} &
  \includegraphics[width=0.12\textwidth]{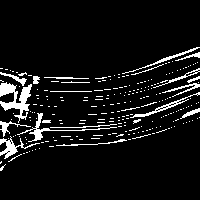} \\
  
 \multirow{2.5}{*}{LiDAR} &
 Prediction & Uncertainty & Error Map & Prediction & Uncertainty & Error Map 
 
 \\
 \cmidrule(lr){2-4}
 \cmidrule(lr){5-7}
 
 & \multicolumn{3}{c}{BEVFusion-L}
 & \multicolumn{3}{c}{MapPrior}
 \\

 \end{tabular}
 \caption{Additional results on uncertainty and error map comparison}
 \label{Additional_Uncertainty Calibration}
 \vspace{-8pt}
 \end{figure*}

\subsection{Failure Cases}
\label{sec:Failure}
Despite the overall improved IoU score in the benchmark, MapPrior can have a lower IoU score than the baseline model in certain cases. 
For example, in Fig.~\ref{fail}, there is a complicated layout distant from the ego car. In such cases, predictive models tend to make empty predictions.
In contrast, MapPrior makes a realistic generation of possible traffic layouts. However, this may lead to significant false positives and a lower IoU score than an empty layout prediction. The better-calibrated confidence score that MapPrior provides should help the downstream planner module be aware of the uncertain areas in this situation. 

 \begin{figure*}[h] \centering 
 \begin{tabular}{ccc}

 \includegraphics[width=0.13\textwidth]{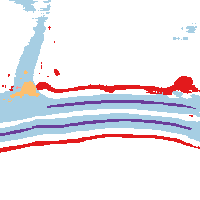}
 &\includegraphics[width=0.13\textwidth]{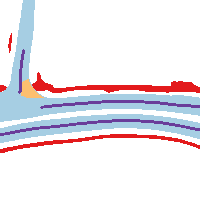}
&\includegraphics[width=0.13\textwidth]{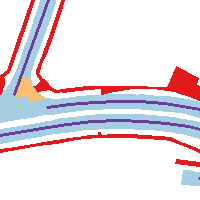}
\\

 \includegraphics[width=0.13\textwidth]{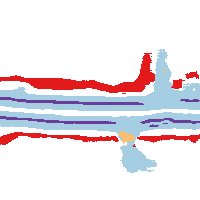}
 &\includegraphics[width=0.13\textwidth]{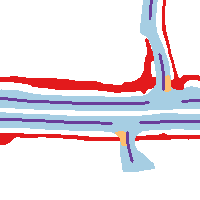}
&\includegraphics[width=0.13\textwidth]{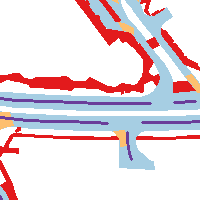}
\\

BEVFusion-L & MapPrior-L (Ours) & GT
 \end{tabular}
 \caption{Failure Cases}

 \label{fail}

 \end{figure*}
