# Supplementary material for: MapPrior: Bird's-Eye View Map Layout Estimation with Generative Models
Source: arXiv:2308.12963 source file (2023-08-24)
Supplement: Supplementary file 3 [file abstract.tex]

\begin{abstract}

In the supplementary material, we provide more qualitative results of BEV map segmentation and uncertainty quantification, as well as additional analysis on failure cases in Sec.~\ref{sec:qual}. 
In addition, we provide model architecture details in Sec.~\ref{sec:arch}. The video "MapPrior.mp4" briefly introduces our task, proposed solution, and compares our results with baseline models.
\end{abstract}
