# Supplementary material for: MapPrior: Bird's-Eye View Map Layout Estimation with Generative Models
Source: arXiv:2308.12963 source file (2023-08-24)
Supplement: Supplementary file 4 [file quant.tex]

\section{Additional Quantitative Results}
\label{sec:quant}

\subsection{Expected calibration error clarification}
We would like to mention that the main paper calculates the expected calibration error (ECE) by evaluating the average rooted mean-squared error between the samples' accuracy and confidence for each bin. This calculation follows the method proposed in "Verified Uncertainty Calibration" \cite{newer_ECE} (Eq. 1). 
Strictly speaking, we should cite Kumar et al.~\cite{newer_ECE} instead of Guo et al.~\cite{ECE_Score} for the ECE calculation. This is because Guo et al. use the mean absolute error instead of the mean squared error, and their ECE score is given by:
$ \texttt{ECE}(B) = \sum_{b=1}^{B} \frac{n_b | \texttt{acc}(b) - \texttt{conf}(b) |_1}{n}.$
We will correct this mis-citation in the next revision of the paper. In addition, to provide a comprehensive understanding, we also compute the original ECE score following Guo et al. \cite{ECE_Score}. Under this metric, our method, MapPrior-L still significantly outperforms the strongest baseline, with scores of 0.021 for MapPrior-L and 0.066 for BEVFusion-L.
